# Supplementary material for: Unidirectional Human-Robot-Human Physical Interaction for Gait Training
Source: arXiv:2409.11510 source file (2024-09-17)
Supplement: Supplementary file 1 [file Old_Additional.tex]

%\begin{figure}[t]
%    \centering
%    \includegraphics[width=1\linewidth]{Exo and IMU Suit v2.png}
%    \caption{a) The 6-DoF Exo-H3 exoskeleton (Technaid S.L., Spain), and b) the IMU suit equipped with 6 IMUs (Tech-IMU V3, Technaid S.L., Spain), and an hub (Tech-HUB V3, Technaid S.L.). In the proposed framework, a patient wears the exoskeleton, while a PT wears the IMU suit. Their joints are haptically connected through a frequency-dependent virtual stiffness.}
%    \label{fig:Exo and IMU suit}
%\end{figure}

%%%%%%%%%%%%%%%%%%%%%%%%%%%%%%%%%%%%%%%%%%%%%%%%%%%%%%%%%%%%%

% Exoskeletons are becoming effective tools in the rehabilitation of patients with lower-limb impairments. However, current control strategies struggle to compensate for the exoskeleton’s whole-body dynamics and to define adequate desired limb trajectories, especially in the case of multi-joint exoskeletons in unstructured scenarios (e.g., obstacles). Moreover, they usually do not allow external physical patient-therapist interaction, reducing the agency of the therapist.

% This work presents a whole-body control (WBC) for a floating-base lower-limb exoskeleton with six active degrees of freedom (DoF), compensating for robot dynamics. The WBC allows the exoskeleton to operate in transparent mode (i.e., zero force interaction), or to render nonzero interaction forces. To define the desired interaction and improve controller stability, we present an interaction control realized with a frequency-dependent stiffness, formulated as a one-pole, one-zero transfer function. Finally, this work proposes a new rehabilitation framework where conventional therapy and robotic exoskeletons are merged together. The therapist, with an inertial measurement unit (IMU) suit, effectively mobilizes all of the patient's limbs at the same time, using unidirectional interaction between the suit and the joints of the patient's exoskeleton. Furthermore, this allow the therapist to adapt to the patient's impairment level and to better target the different rehabilitation scenarios. Results show that the WBC achieved low interaction torques in transparent mode, and that the frequency-dependent stiffness control was more stable than constant stiffness control. Moreover, the IMU-exoskeleton interaction was capable of haptically rendering and transferring joint trajectories from the IMU-user to the exoskeleton-user. The proposed framework can be then considered as an effective tool both in traditional and in more unstructured rehabilitation scenarios.

\begin{figure}[t]
    \centering
    \includegraphics[width=1\linewidth]{Figure 1 Setup v2.png}
    \caption{On the left, a therapist wears the IMU suit equipped with 6 IMUs (Tech-IMU V3, Technaid S.L., Spain), and a hub (Tech-HUB V3, Technaid S.L.). On the right, the 6-DoF Exo-H3 exoskeleton (Technaid S.L., Spain). A patient wears the exoskeleton while a PT wears the IMU suit. Their joints are haptically connected through a unidirectional frequency-dependent virtual stiffness.}
    \label{fig:Exo and IMU suit}
\end{figure}

% Similar approach, where IMU suits or motion capture systems were used to render natural and human-like movements, was explored in the field of teleoperation of humanoid robots \cite{darvish2023teleoperation, stanton2012teleoperation}.


%These gait states are no ground contact (flight), contact by a single foot (single stance), and contact by two feet (double stance). Moreover, the single stance state was divided into right and left stance according to the pressure sensor values. %Figure~\ref{fig:State Machine} presents the state machine structure on gait state estimation and the respective mechanism model with highlighted mass, linkages, and mechanism base frame. 

%\begin{figure}[t]
%    \centering
%    \includegraphics[width=1\linewidth]{StateMachine v3.png}
%    \caption{Gait state machine used in real-time estimation and control. $P_l$ and $P_r$ represent the left and right vertical force readings, respectively. The threshold force used to trigger the state change is $P_{thr}$. For each state, the respective seven-bar linkage model of the exoskeleton is represented, with highlighted mass, linkages, active joints, and mechanism base frame.}
%    \label{fig:State Machine}
%\end{figure}

    $a)$ $Flight:$ The base of the mechanism was assumed to be at the backpack level, with the assumption that during the flight state, the backpack is always aligned vertically with the gravity vector. This assumption is reasonable during normal walking, meaning that the trunk remains straight during walking. In this state, each leg compensates for its own weight, acting independent of one another.

    $b)$ $Single$ $Stance:$ The ankle of the stance leg is assumed to be hinged to the ground, resulting in a seven-link mechanism with six active joints. The stance leg needs to compensate for the weight of the whole exoskeleton. This model results into full exoskeleton weight compensation, backpack included.

    $c)$ $Double$ $Stance:$ The same assumption for the single stance applies, resulting in the summation of the left and right stance model contributions. To deal with both legs a stance interpolation factor ($ \alpha $) was introduced, approximating the double stance state ($\bm{\tau_{\text{grav\_ds}} \in} \mathbb{R}^7$ is the gravity vector) as a transition phase from left stance ($\bm{\tau_{\text{grav\_ls}}}$) to right stance ($\bm{\tau_{\text{grav\_rs}}}$) or vice versa. The total gravity contribution can be expressed as:
\begin{equation}
    \bm{\tau_{\text{grav\_ds}}}=\alpha \bm{\tau_{\text{grav\_ls}}}+(1-\alpha) \bm{\tau_{\text{grav\_rs}}}
\end{equation}
The stance interpolation factor is calculated as the ratio of the left vertical ground reaction force ($P_l$) to the sum of both vertical ground reaction forces ($P_l+P_r$),
\begin{equation}
    \alpha=\frac{P_l}{P_l+P_r}
\end{equation}
This interpolation strategy from left stance to right stance allows smooth continuous modeling of the whole gait cycle during walking \cite{kuccuktabak2023haptic}.

The link masses were experimentally identified with a calibration procedure: exploiting the planar geometry, the gravity contribution was matched in correspondence of several static configuration dependent on a single mass parameter. The adopted methodology was qualitatively similar to \cite{moubarak2010gravity}.


who require more assistance

%On the other hand, exoskeletons should be removed and worn according to different phases of the rehabilitation session.

\begin{figure}[t]
    \centering
    \includegraphics[width=1\linewidth]{StateMachine v3.png}
    \caption{\small Gait state machine. $P_l$ and $P_r$ represent the left and right vertical force readings, respectively. The threshold force used to trigger the state change is $P_{thr}$. For each state, the respective exoskeleton's seven-link mechanism is represented, with highlighted mass, linkages, active joints, and mechanism base frame.}
    \label{fig:State Machine}
\end{figure}


The model accounts for the Coulomb and viscous component of the friction, with a connection region around zero velocities ($\pm\dot{\theta}_{\text{thr}}$) to avoid output discontinuities: 
\begin{equation}
\bm{\textbf{PWM}_{\text{friction}}}= \begin{cases}\bm{c_0}\operatorname{sgn}(\bm{\dot{\theta}})+\bm{c_1}\bm{\dot{\theta}}, & \mbox{if } |\bm{\dot{\theta}}|\geq\dot{\theta}_{\text{thr}} \\ 
\cfrac{\bm{c_0}}{\dot{\theta}_{\text{thr}}}\bm{\dot{\theta}}, & \mbox{if } |\bm{\dot{\theta}}|<\dot{\theta}_{\text{thr}}.
\end{cases}
\end{equation}


However, the definition of appropriate desired limb trajectories is a problem~\cite{belda2011rehabilitation}. %, particularly for multi-joint exoskeletons where each joint requires synergistic and coordinated trajectories ~\cite{belda2011rehabilitation}. 
Approaches where a predefined reference trajectory is computed offline have been proposed in overground walking or in controlled scenarios. In the case of unconstrained or unexpected scenarios (e.g., obstacles), these approaches fail to adapt without a learning phase prior to the event. 
%Moreover, especially in case of patients with very low mobility, it is difficult to achieve appropriate assistance levels (i.e., large torques and impedance control gains) due to limited controller bandwidth~\cite{dalla2021review}.
% but ...
% Often these assistive strategies result in the patient playing a passive role, resulting in a smaller activation of motor learning mechanisms \cite{fray2019evaluation}. 
Furthermore, these devices usually do not allow the therapist to provide external physical guidance as is typical during conventional rehabilitation. By not exploiting the therapist’s knowledge and ability, the agency of the therapist and the efficacy of the rehabilitation is reduced.

In our previous works, we investigated bidirectional physical human-robot-human interactions, both with single-joint connections at the ankle~\cite{short2023haptic} and with multi-joint connections between two lower-limb exoskeletons \cite{kuccuktabak2023virtual}. 


\begin{table}[t]
    \centering
    \caption{\small Results for the constant stiffness ($K_c$) and frequency dependent stiffness ($K_f$) controllers during ...: the first two rows report the average delay as percentage of gait duration (\%) and time (s). The last three rows report the mean absolute interaction torque ($m$Nm/kg) for each joint.}
    \renewcommand{\arraystretch}{1.3}
    \begin{tabular}{p{0.04\textwidth}| c c | c c | c c}
        \hline
         & $K_{c\_0.5}$ & $K_{f\_0.5}$ & $K_{c\_1.1}$ & $K_{f\_1.1}$ & $K_{c\_1.5}$ & $K_{f\_1.5}$\\ [0.5ex]
        \hline
        Delay & 0.25 & 0.35 & 2.95 & 8.05 & 7.60 & 18.70 \\ 
        Delay & 0.016 & 0.022 & 0.098 & 0.266 & 0.201 & 0.494 \\ [0.3ex]
        \hline
        $\overline{\tau}_{\text{hip}}$ & 48$\pm$40 & 49$\pm$37 & 59$\pm$41 & 66$\pm$52 & 85$\pm$47 & 76$\pm$52 \\
        $\overline{\tau}_{\text{knee}}$ & 47$\pm$29 & 45$\pm$31 & 94$\pm$72 & 111$\pm$71 & 117$\pm$77 & 131$\pm$76 \\
        $\overline{\tau}_{\text{ankle}}$ & 35$\pm$19 & 33$\pm$19 & 53$\pm$36 & 48$\pm$32 & 59$\pm$52 & 61$\pm$32 \\ [0.3ex]
        \hline
    \end{tabular}
    \label{tab:playback results table}
    \vspace{-0.2cm}
\end{table}


During our first experiment, we used constant $k_{\text{low\_f}}~=~150$~Nm/rad and $f_{\text{cut}}=1$~Hz, while we varied $k_{\text{high\_f}}$ as listed in Table~\ref{tab:tansfer function values step}.
The 1~Hz frequency was chosen since human movements are usually bounded into this range, while the $k$ values were fine tuned to have a stiff behavior.
Notice that when $k_{\text{high\_f}} = 0$~Nm/rad, the proposed approach results in a low-pass filter applied to the controller's input signal. Otherwise, by setting $k_{\text{high\_f}} = k_{\text{low\_f}} $, the behaviour becomes the one of a constant stiffness along the whole frequency spectrum.
Fig.~\ref{fig:bode plot} shows the Bode plot of the different $K(s)$ tested with the constant stiffness ($K_1$) and the low-pass filter ($K_6$) case. In general, by adding more poles and zeros, or by properly adjusting the $k_{\text{low\_f}}$, $k_{\text{high\_f}}$ and $f_{\text{cut}}$ values, it is possible to limit the interaction to have frequency components that are useful for the rehabilitation program, shifting from low frequencies in the early stages of rehabilitation to high frequencies when the patient is recovering the motor functionality.

Two experiments were then conducted to demonstrate the behavior of the variable impedance controller. In the first experiment, we evaluated the effects of using different set of gains (i.e., $k_{\text{low\_f}}, k_{\text{high\_f}}, f_{\text{cut}}$) on the transient response characteristics for a single joint when imposed a step error as controller input. As mentioned in Section \ref{Interaction Control}, six different $k_{\text{high\_f}}$ values (see Table~\ref{tab:tansfer function values step}) were tested, and to each a step error of 45\textdegree$ $ was commanded to the middle-level controller. The resultant rise time, settling time, and overshoot were recorded. A large step error was chosen to clearly distinguish the effects of each set of gains.
% In fact, even if friction compensation was implemented, residual natural actuator damping can cause the settling in case of little controller dynamics. In particular, in case of the constant stiffness controller, marginal stability was expected due to the absence of a damping term, while in the other cases, the contribution of previous inputs in Eq.~\ref{eq:transfer function} can recall damping terms and lead to improved stability.

% \begin{figure}[t]
%     \centering 
%     % \vspace{0.2cm}
%     \includegraphics[width=0.75\linewidth]{Figure Stability v4.png}
%     \caption{\small Step response results of the different transfer functions tested. The missing bars are not reported due to controller instability. For the overshoot, the $K_1$ controller was marginally stable.}
%     \label{fig:Results stability}
%     \vspace{-0.2cm}
% \end{figure}

In this section, we present the results conducted to evaluate the virtual impedance control on transient response, and subsequently on a treadmill walking test where the user wears the exoskeleton and interacts with a virtual perfect teacher, rendered using prerecorded trajectories.

% Interaction Control Stability (old subsection)
In the first test, we investigated transient response characteristics of different sets of frequency thresholds (Table~\ref{tab:tansfer function values step}). The constant gain controller ($K_1$) and the low-pass filter ($K_6$) were marginally stable and unstable, respectively, while the other parameters resulted in stable responses. 
Considering the rise time, all the controllers have similar behavior ($\overline{t}_{\text{rise}}=$ 0.43$\pm$0.023 s), while for the settling time, $K_2$ and $K_3$ reached the steady state faster than the other conditions ($t_{\text{settling}}=$ 2.04 and 1.95 s respectively). The same considerations apply to the overshoot percentage. %, where $K_2$ resulted in a value of 43.33\%, and $K_3$ of 46.66\%. 
In summary, it is observed that having very small ($K_6$) or very large ($K_1$) high-frequency thresholds may let the controller suffer of instabilities (worse settling time and overshoot values), and thus reduced safety for the exoskeleton user.
% discussion
Moreover, considering the settling time and the overshoot values, it suggests that there is a range of $k_{\text{high\_f}}$ gains, among those tested, for which the controller is more stable, and that therefore stability does not increase by decreasing the gain for high-frequency components as originally assumed. This behavior can be explained by considering the effect of this controller on the torque controller. The transfer function adds a pole and a zero in the overall root locus, and a blind placing of those can lead to instability. 
% A deeper investigation of this aspect will bring a better understanding of the underlying mechanisms.



% \begin{table}[t]
%     \centering
%     \caption{\small Results of the constant stiffness ($K_c$) and frequency dependent stiffness ($K_f$) controllers behaviors for the hip joint, during the treadmill walking test while interacting with a virtual perfect partner. From the first to last row: mean tracking error variation (deg/s); mean interaction torque variation (Nm/kg*s); mean absolute interaction torque ($m$Nm/kg).}
%     \renewcommand{\arraystretch}{1.3}
%     \begin{tabular}{p{0.04\textwidth}| c c | c c | c c}
%         \hline
%          & $K_{c\_0.5}$ & $K_{f\_0.5}$ & $K_{c\_1.1}$ & $K_{f\_1.1}$ & $K_{c\_1.5}$ & $K_{f\_1.5}$\\ [0.5ex]
%         \hline
%         $\overline{\dot{\theta}_{\text{hip\_err}}}$ & 119$\pm$30 & 100$\pm$51 & 77$\pm$35 & 88$\pm$32 & 135$\pm$38 & 141$\pm$12 \\ 
%         $\overline{\dot{\tau}_{\text{hip}}}$ & 1.12$\pm$0.33 & 0.99$\pm$0.48 & 1.11$\pm$0.25 & 0.95$\pm$0.29 & 1.68$\pm$0.38 & 1.39$\pm$0.13 \\
%         $\overline{\tau}_{\text{hip}}$ & 48$\pm$40 & 49$\pm$37 & 59$\pm$41 & 66$\pm$52 & 85$\pm$47 & 76$\pm$52 \\ [0.3ex]
%         \hline
%     \end{tabular}
%     \label{tab:playback results table}
%     \vspace{-0.2cm}
% \end{table}


or use Fig1. As Video 1 (like last paper of A. Young on https://www.science.org/doi/abs/10.1126/scirobotics.adi8852)

 the variable impedance controller resulted in smaller values with respect to the constant stiffness controller (-12\% at 0.5 km/h,-14\% at 1.1 km/h,-17\% at 1.5 km/h) 0.99$\pm$0.48 vs 1.12$\pm$0.33 at 0.5 km/h, 0.95$\pm$0.29 vs 1.11$\pm$0.25 at 1.1 km/h, 1.39$\pm$0.13 vs 1.68$\pm$0.38 at 1.5 km/h)
